# Supplementary material for: Microscale velocity-dependent unbinding generates a macroscale performance-efficiency tradeoff in actomyosin systems
Source: arXiv:2411.02340 source file (2024-11-04)
Supplement: Supplementary file 1 [file supplimental_info.pdf]

# SI Figures

## SI Figure 1

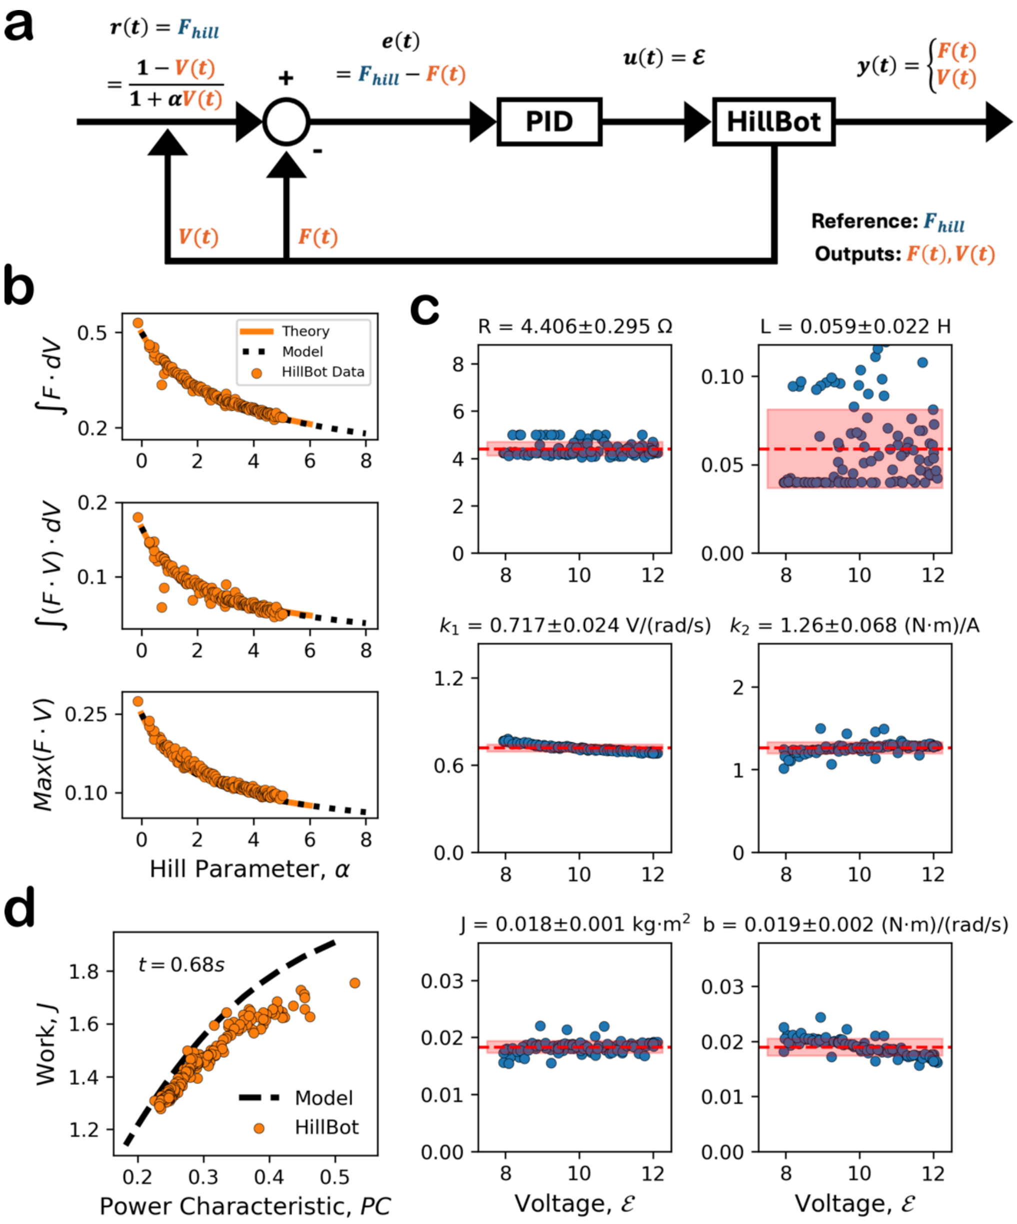


**SI Figure 1:** HillBot system properties. a) Feedback control scheme used to generate nonlinear, Hill-type curves in HillBot for some initialized nonlinearity $\alpha$. The reference signal, $F_{Hill}$, is determined at each loop cycle by HillBot's measured contraction rate $V(t)$ and is compared with its measured force $F(t)$. A PID determines the correct input voltage $\mathcal{E}$ to minimize error between the reference Hill force and measured force, generating nonlinear fv curves. b) For HillBot, the model and Hill's equation, we compare the area under the force- and power-velocity curves in addition to the maximum power value for each tested $\alpha$. HillBot, the model and Hill's equation show strong agreement for all tested values of $\alpha$, providing convincing evidence that HillBot accurately mimics Hill's equation. c) Fitted constants of the system used to integrate equations 10-13. For a range of voltages, we recorded a timeseries of HillBot's current draw and output angular velocity and, using a fitting algorithm, determined the system's constants $\Pi$. d) Increase in HillBot's work output with the power characteristic under a fixed amount of time $t = 0.68s$.

# SI Figure 2

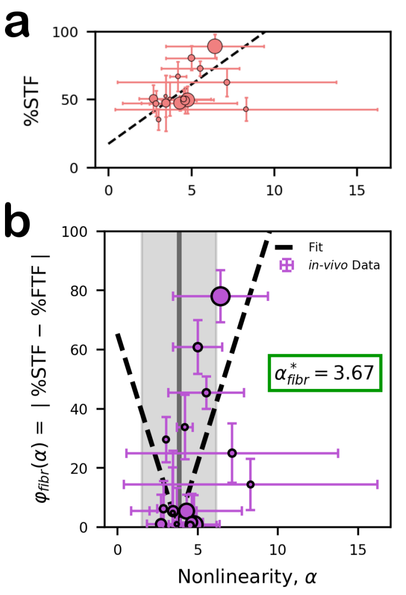


SI Figure 2: A tradeoff in a muscle's share of slow- and fast- twitch muscle fibers is minimized around $\alpha^* = 3.85 \pm 2.32$. a) Scatter plot (red symbols) of percent slow-twitch-fiber composition (%STF) for 16 muscle groups as a function of the Hill nonlinearity parameter $\alpha$. For each muscle group, the %STF data is taken from Ref. [1] ($\pm$ standard deviation across 6 cadavers), and the $\alpha$ data is taken from our meta-analysis ($\pm$ standard deviation across meta-analysis). Symbol size is proportional to number of independent measurements of $\alpha$. Black, dashed line: linear fit, $R^2 = 0.43$. b) Objective function $\phi_{\text{fibr}}$ applied to %STF data (purple symbols) and the linear fit from panel a (black dashed line) as a function of $\alpha$. $\alpha^*_{\text{fibr}} = 3.67$ (green box) minimizes the difference in a muscle's percent composition of slow- and fast-twitch muscle fibers; $\alpha^*_{\text{fibr}} = 3.67$ is within the bounds of $\alpha^* = 3.85 \pm 2.32$ (vertical gray line and region).

Muscle comprises two types of contractile fibers: slow-twitch (Type I) fibers (STF) and fast-twitch (Type-II) fibers (FTF) where a muscle's $\%STF + \%FTF = 100\%$. Muscles with high fractions of STF improve performance in endurance activities [2, 3] and posture maintenance [4], activities where energetic efficiency is vital. Elite endurance runners, for example, hold high fractions of STF [5]. Additionally, muscles with predominately FTF tend to be strong and powerful [6, 3, 7, 8, 9] – with world-class track sprinters [10] and power-lifters [11] possessing high abundance of FTF.

In order to extend the results of HillBot and the 2-state model of actin-myosin dynamics, we continue our meta-analysis to a subset of studies where the composition of muscle fiber types have been measured. Ref. [1] measured the percent composition of slow- and fast- twitch muscle fibers

in 36 different muscle groups across 6 different human male cadavers. For $N = 16$ different muscle groups, we plot the muscle's %STF (as measured by Ref. [1]) against its nonlinearity $\alpha$ (as measured by various sources from the meta-analysis, cf. Fig. 5 and SI Table 3).

We find a positive correlation between a muscle's %STF and the nonlinearity parameter $\alpha$ (SI Fig. 2a). This result agrees with prior observations that slow twitch fibers are more efficient, and that muscle groups with higher values of $\alpha$ are more efficient. However, here we relate %STF and $\alpha$ directly. Conversely, muscle groups with low %STF have high %FTF. The positive correlation in SI Fig. 2 implies that muscle groups with high %FTF are correlated with lower values of $\alpha$, consistent with previous evidence that fast twitch fibers and low $\alpha$-valued muscle groups are powerful. We therefore expect muscle's performance-economy tradeoff to be reflected in an exchange of muscle fiber type composition.

To determine how $\alpha$ affects this tradeoff in terms of fiber type composition, we construct again an objective function $\phi_{\mathrm{fibr}}$. This time, $\phi_{\mathrm{fibr}}(\alpha) := |\%STF(\alpha) - \%FTF(\alpha)| = |100\% - 2 \cdot \%STF(\alpha)|$ depends on the relationship between %STF and $\alpha$, which we determine by a linear fit (SI Fig. 2a, black dashed line, $R^2 = 0.43$). We find a non-monotonic dependence of $\phi_{\mathrm{fibr}}$ on $\alpha$ (SI Fig. 2b), with a minimum at $\alpha^*_{\mathrm{fibr}} = 3.67$. This result demonstrates that variations in $\alpha$ reflect a tradeoff between performance and economy in muscle via muscle-fiber-type composition. Furthermore, we again observe that $\alpha^*_{\mathrm{fibr}} = 3.67$ agrees with the characteristic value of $\alpha^* = 3.85 \pm 2.32$ that we observed in our earlier meta-analysis (cf. Fig. 5e). Finally, we note a large grouping of muscles at $\alpha \approx 4$, corresponding to a 50% STF composition, suggesting that an even distribution of STF and FTF fibers favors both efficiency and power output. It is important to note, however, that fiber types are recruited dependent on task demands [12] by Henneman's size principle.

## SI Fig. 2 References


[1] M. A. Johnson, J. Polgar, D. Weightman, and D. Appleton. Data on the distribution of fibre types in thirty-six human muscles: An autopsy study. *Journal of the Neurological Sciences*, 18(1):111–129, January 1973. Publisher: Elsevier.

[2] J. F. Horowitz, L. S. Sidossis, and E. F. Coyle. High Efficiency of Type I Muscle Fibers Improves Performance. *Int J Sports Med*, 15(3):152–157, April 1994. Publisher: © Georg Thieme Verlag Stuttgart · New York.

[3] Jacob M. Wilson, Jeremy P. Loenneke, Edward Jo, Gabriel J. Wilson, Michael C. Zourdos, and Jeong-Su Kim. The Effects of Endurance, Strength, and Power Training on Muscle Fiber Type Shifting. *The Journal of Strength & Conditioning Research*, 26(6):1724, June 2012.

[4] Yoshiaki Hitomi, Takako Kizaki, Sumiko Watanabe, George Matsumura, Yasunori Fujioka, Shukoh Haga, Tetsuya Izawa, Naoyuki Taniguchi, and Hideki Ohno. Seven skeletal muscles rich in slow muscle fibers may function to sustain neutral position in the rodent hindlimb. *Comparative Biochemistry and Physiology Part B: Biochemistry and Molecular Biology*, 140(1):45–50, January 2005.

[5] P. A. Tesch and J. Karlsson. Muscle fiber types and size in trained and untrained muscles of elite athletes. *Journal of Applied Physiology*, 59(6):1716–1720, December 1985. Publisher: American Physiological Society.

[6] Andrew C. Fry, Jesse M. Webber, Lawrence W. Weiss, Matthew P. H Arber, Mark Vaczi, and Nancy A. Pattison. Muscle Fiber Characteristics of Competitive Power Lifters. *The Journal of Strength & Conditioning Research*, 17(2):402, May 2003.

[7] Pierre Samozino, Enrico Rejc, Pietro Prampero, Alain Belli, and Jean-Benoît Morin. Optimal Force–Velocity Profile in Ballistic Movements—Altius. *Medicine and science in sports and exercise*, 44:313–22, July 2011.

[8] Pierre Samozino, Nicolas Peyrot, Pascal Edouard, Ryu Nagahara, Pedro Jimenez-Reyes, Bene-

dicte Vanwanseele, and Jean-Benoit Morin. Optimal mechanical force-velocity profile for sprint acceleration performance. *Scandinavian Journal of Medicine & Science in Sports*, 32(3):559–575, 2022.

[9] Andrés Baena-Raya, Pablo García-Mateo, Amador García-Ramos, Manuel A. Rodríguez-Pérez, and Alberto Soriano-Maldonado. Delineating the potential of the vertical and horizontal force-velocity profile for optimizing sport performance: A systematic review. *Journal of Sports Sciences*, February 2022. Publisher: Routledge.

[10] Scott Trappe, Nicholas Luden, Kiril Minchev, Ulrika Raue, Bozena Jemiolo, and Todd A. Trappe. Skeletal muscle signature of a champion sprint runner. *Journal of Applied Physiology*, 118(12):1460–1466, June 2015. Publisher: American Physiological Society.

[11] Nathan Serrano, Lauren M. Colenso-Semple, Kara K. Lazauskus, Jeremy W. Siu, James R. Bagley, Robert G. Lockie, Pablo B. Costa, and Andrew J. Galpin. Extraordinary fast-twitch fiber abundance in elite weightlifters. *PLOS ONE*, 14(3):e0207975, March 2019. Publisher: Public Library of Science.

[12] Elwood Henneman. Relation between Size of Neurons and Their Susceptibility to Discharge. *Science*, December 1957. Publisher: American Association for the Advancement of Science.

# SI Tables

## SI Table 1

Lookup table of variables, their representation, values and respective formulas.

| Variable | Representation | Value |
|---|---|---|
| Hill parameter / nonlinearity | $\alpha$ | --- |
| Characteristic nonlinearity | $\alpha^*$ | $\alpha^* = 3.85 \pm 2.32$ |
| Optimal nonlinearity in HillBot | $\alpha^*_{bot}$ | $\alpha^*_{bot} = 4.0$ |
| Optimal nonlinearity in 2-state model | $\alpha^*_{2-st}$ | $\alpha^*_{2-st} = 5.66$ |
| Optimal nonlinearity in fiber-type composition | $\alpha^*_{fibr}$ | $\alpha^*_{fibr} = 3.67$ |
| Power characteristic | $PC$ | $PC = \int F \cdot dV$ |
| Applied voltage | $\mathcal{E}$ | --- |
| Normalized voltage / voltage | $V^-$ | $V^- = \mathcal{E}/12.0$ |
| Measured current | $i$ | --- |
| Measured force | $f$ | $f = 0.544 \cdot (i - 0.022)\ {}^{N}/_{m}$ |
| Measured velocity | $v$ | --- |
| Maximum velocity | $v_m$ | $v_m = 15.71\ {}^{rad}/_{s}$ |
| Maximum current draw | $i_m$ | $i_m = 2.95\ A$ |
| Maximum force | $f_m$ | $f_m = 1.59\ N/m$ |
| Initial current draw | $i_0$ | --- |
| Steady state current | $i_s$ | $i_s = 0.014 \cdot \mathcal{E} + 0.068\ A$ |
| Motor constant | $C$ | $C = \frac{i_0}{i_m}$ |
| Normalized current | $I$ | $I = i/i_m$ |
| Normalized force | $F$ | $F = f/f_m$ |
| Normalized velocity | $V$ | $V = v/v_m$ |
| Circuit resistance | $R$ | $R = 4.4060 \pm 0.2949\ \Omega$ |
| Motor Inductance | $L$ | $L = 0.0589 \pm 0.0223\ H$ |
| Motor back emf-velocity proportionality constant | $k_1$ | $k_1 = 0.7169 \pm 0.0239\ \frac{V}{{}^{rad}/_{s}}$ |
| Motor torque-current proportionality constant | $k_2$ | $k_2 = 1.2605 \pm 0.0684\ \frac{{}^{N}/_{m}}{A}$ |
| Motor moment of inertia | $J$ | $J = 0.0183 \pm 0.0010\ kg \cdot m^2$ |
| Motor damping constant | $b$ | $b = 0.0190 \pm 0.0016\ N \cdot {}^{m}/_{s}$ |

# SI Table 2

Meta-analysis results.

| Animal | Nickname | Muscle | Hill parameter | Temperature (C) | Average? | Reference |
|---|---|---|---|---|---|---|
| Homo Sapien | Human | Adductor Pollicis | 3.571428571 | 36 | Yes | de Ruiter 1999 |
| Homo Sapien | Human | Adductor Pollicis | 5 | 36 | Yes | de Ruiter 1999 |
| Homo Sapien | Human | Adductor Pollicis | 4.347826087 | 36 | Yes | de Ruiter 2000 |
| Homo Sapien | Human | Adductor Pollicis | 7.142857143 | 36 | Yes | de Ruiter 2000 |
| Mytilus edulis | Blue mussel | Anterior byssus retractor | 14.28571429 | 20 | Yes | Gilbert 1978 |
| Gallus gallus | Chicken | Anterior latissimus dorsi | 9.090909091 | 21 | Yes | Rall 1973 |
| Homo sapien | Human | Biceps brachii | 2.127659574 | | Yes | Valour 2003 |
| Homo sapien | Human | Biceps brachii | 1.960784314 | | Yes | Valour 2003 |
| Homo sapien | Human | Biceps brachii | 2.272727273 | | Yes | Valour 2003 |
| Homo sapien | Human | Biceps brachii | 3.03030303 | | Yes | Valour 2003 |
| Homo sapien | Human | Biceps brachii | 2.564102564 | | Yes | Valour 2003 |
| Homo sapien | Human | Biceps brachii | 4.347826087 | | Yes | Valour 2003 |
| Homo sapien | Human | Biceps femoris | 4.545454545 | | | Miller 2016 |
| Felis catus | House cat | Extensor digitorum longus | 14.83928571 | | Yes | Baratta 1995 |
| Mus musculus | Mouse | Extensor digitorum longus | 2.145922747 | 25 | Yes | Barclay 1996 |
| Mus musculus | Mouse | Extensor digitorum longus | 1.543209877 | 25 | Yes | Barclay 1996 |
| Mus musculus | Mouse | Extensor digitorum longus | 2.941176471 | 21 | Yes | Barclay 1993 |
| Mus musculus | Mouse | Extensor digitorum longus | 3.571428571 | | | Houdijk 2006 |
| Mus musculus | Mouse | Extensor digitorum longus | 3.571428571 | | | Houdijk 2006 |
| Rattus | Rat | Extensor digitorum longus | 3.225806452 | 35 | Yes | Ranatunga 1990 |
| Rattus | Rat | Extensor digitorum longus | 6.993006993 | 10 | Yes | Ranatunga 1984 |
| Rattus | Rat | Extensor digitorum longus | 5.263157895 | 15 | Yes | Ranatunga 1984 |
| Rattus | Rat | Extensor digitorum longus | 3.745318352 | 20 | Yes | Ranatunga 1984 |
| Rattus | Rat | Extensor digitorum longus | 2.7100271 | 25 | Yes | Ranatunga 1984 |
| Rattus | Rat | Extensor digitorum longus | 2.906976744 | 30 | Yes | Ranatunga 1984 |
| Rattus | Rat | Extensor digitorum longus | 2.604166667 | 35 | Yes | Ranatunga 1984 |
| Felis catus | House cat | Flexor digitorum longus | 5.601785714 | | Yes | Baratta 1995 |
| Homo sapien | Human | Flexor digitorum longus | 3.03030303 | | | Wilke 1949 |
| Homo sapien | Human | Flexor digitorum longus | 2.083333333 | | | Wilke 1949 |
| Homo sapien | Human | Flexor digitorum longus | 2.380952381 | | | Wilke 1949 |
| Homo sapien | Human | Flexor digitorum longus | 2.702702703 | | | Wilke 1949 |
| Homo sapien | Human | Flexor digitorum longus | 5 | | | Wilke 1949 |
| Homo Sapien | Human | Forearms | 3 | | | Hill 1940 |
| | Human | Forearms | 4 | | | Hill 1940 |
| Homo Sapien | Human | Forearms | 5 | | | Hill 1940 |
| Homo sapien | Human | Gastrocnemius | 3.333333333 | | | Miller 2016 |
| Felis catus | House cat | Gastrocnemius lateral | 6.415238095 | | Yes | Baratta 1995 |
| Felis catus | House cat | Gastrocnemius medial | 3.861111111 | | Yes | Baratta 1995 |
| Homo sapien | Human | Glutei | 3.448275862 | | | Miller 2016 |
| Homo sapien | Human | Hamstrings | 3.846153846 | | | Miller 2016 |
| Xenopus laevis | African clawed frog | Iliofibularis | 2.325581395 | 20 | Yes | Buschman 1997 |
| Xenopus Laevis | African clawed frog | Iliofibularis | 2.631578947 | 20 | Yes | Lannergren 1978 |
| Xenopus Laevis | African clawed frog | Iliofibularis | 2.857142857 | 10 | Yes | Lannergren 1978 |
| Xenopus Laevis | African clawed frog | Iliofibularis | 2.857142857 | 5 | Yes | Lannergren 1978 |
| Xenopus Laevis | African clawed frog | Iliofibularis | 10 | 22 | | Lannergren 1978 |
| Xenopus Laevis | African clawed frog | Iliofibularis | 3.125 | 20 | Yes | Lännergren 1987 |
| Xenopus Laevis | African clawed frog | Iliofibularis | 3.448275862 | 20 | Yes | Lännergren 1987 |
| Xenopus Laevis | African clawed frog | Iliofibularis | 3.846153846 | 20 | Yes | Lännergren 1987 |

| | | | | | | |
|---|---|---|---|---|---|---|
| Xenopus Laevis | African clawed frog | Iliofibularis | 4.761904762 | 20 | Yes | Lännergren 1987 |
| Pseudemys scripta | Pond slider | Iliofibularis | 3.448275862 | 5 | Yes | Mutungi 1987 |
| Pseudemys scripta | Pond slider | Iliofibularis | 3.03030303 | 15 | Yes | Mutungi 1987 |
| Pseudemys scripta | Pond slider | Iliofibularis | 2.43902439 | 5 | Yes | Mutungi 1987 |
| Homo sapien | Human | Iliopsoas | 3.225806452 | | | Miller 2016 |
| Squalus acabthias | Dogfish | White myotome | 4.166666667 | 12 | | Curtin 1991 |
| Cayprinus carpio | Carp | Red myotome | 2.040816327 | 10 | Yes | Rome 1990 |
| Cayprinus carpio | Carp | Red myotome | 3.448275862 | 20 | Yes | Rome 19990 |
| Felis catus | House cat | Peroneus brevis | 6.45 | | Yes | Baratta 1995 |
| Felis catus | House cat | Peroneus longus | 14.74285714 | | Yes | Baratta 1995 |
| Meleagris | Wild turkeys | Peroneus longus | 3.846153846 | 20 | Yes | Nelson 2004 |
| Rattus | Rat | Peroneus longus | 2.857142857 | 35 | Yes | Ranatunga 1990 |
| Gallus gallus | Chicken | Posterior latissimus dorsi | 3.703703704 | | Yes | Rall 1973 |
| Oryctolagus Cuniculus | Rabbit | Psoas | 4.347826087 | 10 | | Cooke 1988 |
| Oryctolagus Cuniculus | Rabbit | Psoas | 4.545454545 | 10 | | Cooke 1988 |
| Oryctolagus Cuniculus | Rabbit | Psoas | 5 | 10 | | Cooke 1988 |
| Oryctolagus Cuniculus | Rabbit | Psoas | 5 | 10 | | Cooke 1988 |
| Oryctolagus Cuniculus | Rabbit | Psoas | 5.263157895 | 10 | | Cooke 1988 |
| Oryctolagus Cuniculus | Rabbit | Psoas | 5 | 10 | | Cooke 1988 |
| Homo sapien | Human | Rectus femoris | 2.702702703 | | | Miller 2016 |
| Testudo hermanni | Greek tortoise | Rectus femoris | 13.88888889 | 0 | Yes | Woledge 1968 |
| Rana temporaria | Common frog | Sartorius | 4.902777778 | | | Alcazar 2019 |
| Rana temporaria | Common frog | Sartorius | 3.621621622 | | | Alcazar 2019 |
| Rana pipiens | Northern leopard frog | Sartorius | 9.090909091 | | Yes | Gilbert 1986 |
| Rana pipiens | Northern leopard frog | Sartorius | 5.555555556 | | Yes | Gilbert 1986 |
| Rana pipiens | Northern leopard frog | Sartorius | 6.666666667 | | Yes | Gilbert 1986 |
| Rana pipiens | Northern leopard frog | Sartorius | 3.846153846 | | Yes | Gilbert 1986 |
| Rana temporaria | Common frog | Sartorius | 3.891050584 | 0 | | Hill 1938 |
| Rana temporaria | Common frog | Sartorius | 3.571428571 | 8.9 | | Hill 1938 |
| Rana temporaria | Common frog | Sartorius | 3.448275862 | 13.5 | | Hill 1938 |
| Rana temporaria | Common frog | Sartorius | 5.555555556 | 19.8 | | Hill 1938 |
| Rana temporaria | Common frog | Sartorius | 5.263157895 | 13 | | Hill 1938 |
| Rana temporaria | Common frog | Sartorius | 6.666666667 | | | Hill 1964 |
| Rana temporaria | Common frog | Sartorius | 5 | | | Hill 1964 |
| Rana temporaria | Common frog | Sartorius | 4 | | | Hill 1964 |
| Rana temporaria | Common frog | Sartorius | 3.333333333 | | | Hill 1964 |
| Rana temporaria | Common frog | Sartorius | 2.857142857 | | | Hill 1964 |
| Rana temporaria | Common frog | Sartorius | 4 | | | Hill 1939 |
| Carcinus maenas | European green crab | Scaphoganthite levator | 2.43902439 | 15 | | Josephson 1987 |
| Mus Musculus | Mouse | Soleus | 6.666666667 | 20 | | Asmussen 1989 |
| Rattus | Rat | Soleus | 3.03030303 | 20 | | Asmussen 1989 |
| Cavia Porcellus | Guinea-Pig | Soleus | 10 | 20 | | Asmussen 1989 |
| Felis catus | House cat | Soleus | 1.078424658 | | Yes | Baratta 1995 |
| Mus musculus | Mouse | Soleus | 6.134969325 | | Yes | Barclay 1993 |
| Mus musculus | Mouse | Soleus | 4.830917874 | | Yes | Barclay 1993 |
| Mus musculus | Mouse | Soleus | 7.042253521 | | Yes | Barclay 1993 |
| Rattus | Rat | Soleus | 7.142857143 | 30 | | Caiozzo 1991 |
| Rattus | Rat | Soleus | 13.33333333 | 20 | | Clafin 1989 |
| Mus musculus | Mouse | Soleus | 6.25 | | | Houdijk 2006 |
| Mus musculus | Mouse | Soleus | 6.25 | | | Houdijk 2006 |
| Homo sapien | Human | Soleus | 5.555555556 | | | Miller 2016 |
| Rattus | Rat | Soleus | 3.846153846 | 35 | Yes | Ranatunga 1990 |
| Rattus | Rat | Soleus | 11.82033097 | 10 | Yes | Ranatunga 1984 |
| Rattus | Rat | Soleus | 9.009009009 | 15 | Yes | Ranatunga 1984 |
| Rattus | Rat | Soleus | 6.329113924 | 20 | Yes | Ranatunga 1984 |
| Rattus | Rat | Soleus | 4.830917874 | 25 | Yes | Ranatunga 1984 |
| Rattus | Rat | Soleus | 4.854368932 | 30 | Yes | Ranatunga 1984 |
| Rattus | Rat | Soleus | 4.201680672 | 35 | Yes | Ranatunga 1984 |
| Rattus | Rat | Sternomastoid | 3.039513678 | | Yes | Luff 1985 |
| Rattus | Rat | Sternomastoid | 3.03030303 | | Yes | Luff 1985 |
| Rana temporaria | Common frog | Tibialis anterior | 3.5 | | | Alcazar 2019 |
| Felis catus | House cat | Tibialis anterior | 8.126388889 | | Yes | Baratta 1995 |
| Homo sapien | Human | Tibialis anterior | 5 | | | Miller 2016 |
| Felis catus | House cat | Tibialis posteriror | 11.03611111 | | Yes | Baratta 1995 |
| Homo sapien | Human | Vasti | 2.941176471 | | | Miller 2016 |
| Homo sapien | Human | Vastus lateralis | 2.43902439 | | Yes | Tihanyi 1982 |
| Homo sapien | Human | Vastus lateralis | 3.225806452 | | Yes | Tihanyi 1982 |
| Scyliorhinus canicula | Dogfish | White myotome | 2.78913738 | 12 | Yes | Curtin 1991 |
| Makaira nigricans | Marlin | Red myotome | 4.166666667 | 15 | | Johnston 1984 |

| | | | | | | |
|---|---|---|---|---|---|---|
| Makaira nigricans | Marlin | Red myotome | 4.347826087 | 25 | | Johnston 1984 |
| Makaira nigricans | Marlin | White myotome | 8.333333333 | 15 | | Johnston 1984 |
| Makaira nigricans | Marlin | White myotome | 8.333333333 | 25 | | Johnston 1984 |
| Neoconocephalus triops | Broad-tipped conehead | Metathoracic | 1.111111111 | 35 | | Josephston 1984 |
| Neoconocephalus triops | Broad-tipped conehead | Mesothoracic | 0.485436893 | 35 | | Josephston 1984 |
| Neoconocephalus robustus | Robust conehead | Metathoracic | 0.980392157 | 35 | | Josephston 1984 |
| Neoconocephalus robustus | Robust conehead | Mesothoracic | 0.571428571 | 35 | | Josephston 1984 |
| Schistocerca gregaria | Desert locust | Metathoracic | 5 | 30 | | Malamud 1988 |
| Schistocerca americana | American bird grasshopper | Metathoracic | 1.724137931 | 25 | | Malamud 1988 |
| Stenotomus chrysops | Scup | Red myotome | 4 | 10 | | Rome 1992 |
| Stenotomus chrysops | Scup | Red myotome | 4 | 20 | | Rome 1992 |
| Cyprinus carpio | Carp | Red myotome | 3.225806452 | 10 | | Rome 1992 |
| Cyprinus carpio | Carp | Red myotome | 1.960784314 | 20 | | Rome 1992 |
| Cyprinus carpio | Carp | Red myotome | 3.333333333 | 10 | | Rome 1992 |
| Cyprinus carpio | Carp | Red myotome | 2.197802198 | 20 | | Rome 1992 |
| | | Simulation | 4 | | | Romero 2016 |
| | | Simulation | 5 | | | Winters 1995 |
| | | Simulation | 2.5 | | | Winters 1995 |

# SI Table 3

STF-FTF meta-analysis results.

| Muscle | Hill parameter | Hill error | Percent STF | STF error | STF reference | α sample size |
|---|---|---|---|---|---|---|
| Adductor pollicis | 5.01 | 1.53 | 80.4 | 9.1 | Johnson 1973 | 4 |
| Biceps brachii | 2.72 | 0.88 | 50.5 | 10 | Johnson 1973 | 6 |
| Biceps femoris | 4.2 | 0.49 | 66.9 | 10.9 | Johnson 1973 | 2 |
| Extensor digitorum longus | 4.31 | 3.45 | 47.3 | 5.5 | Johnson 1973 | 13 |
| Flexor digitorum profundis | 3.47 | 1.47 | 47.3 | 20.45 | Johnson 1973 | 6 |
| Gastrocnemius | 4.54 | 1.65 | 50.3 | 6.95 | Johnson 1973 | 3 |
| Gluteus maximus | 3.45 | 0 | 52.4 | 15.35 | Johnson 1973 | 1 |
| Iliopsoas | 4.63 | 0.69 | 49.2 | 9.65 | Johnson 1973 | 7 |
| Peroneus longus | 7.15 | 6.6 | 62.5 | 10.05 | Johnson 1973 | 3 |
| Posterior latissimus dorsi | 3.7 | 0 | 50.5 | 12.3 | Johnson 1973 | 1 |
| Rectus femoris | 8.3 | 7.91 | 42.8 | 8.7 | Johnson 1973 | 2 |
| Sartorius | 4.78 | 1.59 | 49.6 | 10.05 | Johnson 1973 | 17 |
| Soleus | 6.43 | 2.96 | 89 | 8.85 | Johnson 1973 | 19 |
| Sternomastoid | 3.03 | 0.007 | 35.2 | 7.65 | Johnson 1973 | 2 |
| Tibialis anterior | 5.54 | 2.36 | 72.7 | 5.45 | Johnson 1973 | 3 |
| Vastus lateralis | 2.87 | 0.4 | 46.9 | 9.35 | Johnson 1973 | 3 |

# SI Table 4

*In-vivo* efficiency meta-analysis results.

| Animal | Muscle | Hill parameter | Hill error | Max efficiency | Efficiency error | Source |
|---|---|---|---|---|---|---|
| Testudo hermanni | Rectus femoris | 13.88888889 | 1.543209877 | 0.76875 | 0.0658 | Woledge 1968 |
| Rana temporaria | Sartorius | 6.666666667 | | 0.404 | | Hill 1964 |
| Rana temporaria | Sartorius | 5 | | 0.422 | | Hill 1964 |
| Rana temporaria | Sartorius | 4 | | 0.429 | | Hill 1964 |
| Rana temporaria | Sartorius | 3.333333333 | | 0.432 | | Hill 1964 |
| Rana temporaria | Sartorius | 2.857142857 | | 0.435 | | Hill 1964 |
| Mus musculus | Extensor digitorum longus | 2.145922747 | 0.262484113 | 0.333 | 0.02 | Barclay 1996 |
| Mus musculus | Extensor digitorum longus | 1.543209877 | 0.221479195 | 0.282 | 0.021 | Barclay 1996 |
| Mus musculus | Soleus | 6.134969325 | 0.376378486 | 0.425 | 0.025 | Barclay 1996 |
| Mus musculus | Soleus | 4.830917874 | 0.513430885 | 0.387 | 0.025 | Barclay 1996 |
| Mus musculus | Soleus | 7.042253521 | 0.694306685 | 0.306 | 0.026 | Barclay 1993 |

| | | | | | | |
|---|---|---|---|---|---|---|
| Mus musculus | Extensor digitorum longus | 2.941176471 | 0.173010381 | 0.283 | 0.024 | Barclay 1993 |
| Mus musculus | Soleus | 6.25 | | 0.459 | | Houdijk 2006 |
| Mus musculus | Soleus | 6.25 | | 0.437 | | Houdijk 2006 |
| Mus musculus | Extensor digitorum longus | 3.571428571 | | 0.318 | | Houdijk 2006 |
| Mus musculus | Extensor digitorum longus | 3.571428571 | | 0.327 | | Houdijk 2006 |
| Rana temporaria | Sartorius | 4 | | 0.405 | | Hill 1939 |
| Rana pipiens | Sartorius | 9.090909091 | 0.826446281 | 0.565947242 | 0.0208 | Gilbert 1986 |
| Rana pipiens | Sartorius | 5.555555556 | 0.617283951 | 0.536 | 0.0209 | Gilbert 1986 |
| Rana pipiens | Sartorius | 6.666666667 | 0.888888889 | 0.422535211 | 0.0194 | Gilbert 1986 |
| Rana pipiens | Sartorius | 3.846153846 | 0.295857988 | 0.40077821 | 0.0171 | Gilbert 1986 |
| Xenopus laevis | Iliofibularis | 2.325581395 | 1.352082207 | 0.33 | 0.02 | Buschman 1997 |
| Mytilus edulis | Anterior byssus retractor | 14.28571429 | 2.040816327 | 0.675 | 0.105 | Gilbert 1978 |
| Scyliorhinus canicula | White myotomal | 2.78913738 | 0.4132 | 0.33 | 0.01 | Curtin 1991 |
| Gallus gallus | Posterior latissimus dorsi | 3.703703704 | 0.137174211 | 0.44 | 0.03 | Rall 1973 |
| Gallus gallus | Anterior latissimus dorsi | 9.090909091 | 0.165289256 | 0.55 | 0.04 | Rall 1973 |

## Derivations

$$
\begin{aligned}
PC_{nl} &= \int_0^1 F_{nl} \cdot dV = \int_0^1 \frac{1-V}{1+\alpha V} \cdot dV \\
PC_l &= \int_0^C F_l \cdot dV = \int_0^C (C-V) \cdot dV
\end{aligned} \tag{1}
$$

$$
\begin{aligned}
PC_l &= PC_{nl} \\
\int_0^C (C-V) \cdot dV &= \int_0^1 \frac{1-V}{1+\alpha V} \cdot dV \\
\frac{C^2}{2} &= \frac{(1+\alpha) \cdot \ln(1+\alpha) - \alpha}{\alpha^2}
\end{aligned} \tag{2}
$$

$$
C = \frac{\sqrt{2}}{\alpha} \sqrt{(1+\alpha) \cdot \ln(1+\alpha) - \alpha} \tag{3}
$$
